# Supplementary material for: MILA: Multi-Task Learning from Videos via Efficient Inter-Frame Attention
Source: arXiv:2002.07362 source file (2021-10-10)
Supplement: Supplementary file 1 [file supp_2.tex]

% \documentclass[10pt,twocolumn,letterpaper]{article}

% \usepackage{iccv}
% \usepackage{times}
% \usepackage{epsfig}
% \usepackage{graphicx}
% \usepackage{amsmath}
% \usepackage{amssymb}

% \usepackage{multirow}
% \usepackage{subcaption}
% \usepackage{booktabs}
% \usepackage{caption}
% \usepackage{subcaption}
% \renewcommand\thesection{\Alph{section}}
% \renewcommand\thetable{\Alph{table}}
% \usepackage[accsupp]{axessibility}
% \graphicspath{{./imgs/}} % to change the path for images
% % Include other packages here, before hyperref.

% % If you comment hyperref and then uncomment it, you should delete
% % egpaper.aux before re-running latex.  (Or just hit 'q' on the first latex
% % run, let it finish, and you should be clear).
% \usepackage[pagebackref=true,breaklinks=true,letterpaper=true,colorlinks,bookmarks=false]{hyperref}

% \iccvfinalcopy % *** Uncomment this line for the final submission

% \def\iccvPaperID{11} % *** Enter the ICCV Paper ID here
% \def\httilde{\mbox{\tt\raisebox{-.5ex}{\symbol{126}}}}

% % Pages are numbered in submission mode, and unnumbered in camera-ready
% \ificcvfinal\pagestyle{empty}\fi
% \newcommand*{\affaddr}[1]{#1} % No op here. Customize it for different styles.
% \newcommand*{\affmark}[1][*]{\textsuperscript{#1}}


% \begin{document}

% %%%%%%%%% TITLE
% \title{Supplementary Material for MILA: Multi-Task Learning from Videos via Efficient Inter-Frame Attention}

% \author{%
%   Donghyun Kim\affmark[1], Tian Lan\affmark[2], Chuhang Zou\affmark[2], Ning Xu\affmark[2], 
%   \\Bryan A. Plummer\affmark[1], Stan Sclaroff\affmark[1], Jayan Eledath\affmark[2], Gerard Medioni\affmark[2]  \\ 
%   \affaddr{\affmark[1]Boston University}, \affaddr{\affmark[2] Amazon}\\
%   \tt\small $^1$\{donhk, bplum, sclaroff\}@bu.edu, $^2$\{tianlan, ninxu, zouchuha, eledathj, medioni\}@amazon.com}

% \maketitle
% % Remove page # from the first page of camera-ready.
% \ificcvfinal\thispagestyle{empty}\fi

% \section{Experiment Details for Fair Comparison}
% As stated in Sec.4.2 in the main paper, for fair comparison to other methods (MTAN~\cite{liu2019end}, Cross-Stitch~\cite{misra2016cross} and MultiNet++~\cite{chennupati2019multinet++}), we unify the backbone for all method as Deeplab-ResNet101~\cite{chen2017deeplab,He_2016_CVPR}. Note that after using Deeplab-ResNet101, the performance for MTAN, Cross-Stitch and MultiNet++ gets improved compared to their originally reported numbers as shown in Table~\ref{tab:cityscapes_sup}. Deeplab-ResNet101 is initialized with pre-trained weights on ImageNet but decoders use randomly initialized weights. Then, the model is finetuned for multi-task learning.

% For implementation details, since all multi-task learning models except Cross-Stitch use shared encoder, we pre-train a shared multi-task encoder based on Deeplab-ResNet101 for each method (named as``D101-MultiTask''). For the Cross-Stitch model we pre-train a task specific encoder~(named as ``D101-SingleTask''). Using networks pre-trained on multi-task learning shows better performances than just directly finetuning pre-trained weights on ImageNet~\cite{gao2019nddr}. We first train D101-SingleTask and D101-MultiTask with Adam optimizer with learning~\cite{kingma2014adam} rate $1e^{-4}$ with a decay rate $1e^{-1}$. For our SlowFast based network, we use the D101-MultiTask for our slow network. We also train a D18-MultiTask for the $Fast$ network with the same optimizer and training setting. For fair comparison with MultiNet++, we use the same pre-trained slow-fast network for MultiNet++, but concatenate neighboring frames as input to learn from videos as proposed in their paper.

% Note that we also report in the main paper the performance comparison with our pre-trained ``D101-SingleTask'' and ``D101-MultiTask''.

% \begin{table}[t]
% \centering
% \small
% \setlength{\tabcolsep}{3.0pt}
% \begin{tabular}{|l|c|c|c|c|}
% \hline
% \multirow{2}{*}{Model}                                                  & \multicolumn{2}{c|}{Segmentation} & \multicolumn{2}{c|}{Depth}  \\ 
% \cline{2-5}
% & mIOU $\uparrow$ & Acc. $\uparrow$ & Abs.  $\downarrow$ & Rel. $\downarrow$  \\ \hline \hline

% MTAN-SegNet~\cite{liu2019end}  & 53.0 & 91.1 & 1.44 & 33.6  \\
% MTAN-ResNet101 & \textbf{64.2} & \textbf{94.5} & \textbf{1.06} & \textbf{26.3}  \\
% Cross-Stitch-SegNet~\cite{liu2019end} & 50.1 & 90.3 & 1.54 & 34.5\\
% Cross-Stitch-ResNet101 & \textbf{64.5} & \textbf{94.5} & \textbf{1.04} & \textbf{33.0} \\
% \hline
% \end{tabular}
% % \vskip 0.1in
% \caption{Comparison of different backbones. Using the ResNet101 backbone improves the accuracy by a large margin.}
% \label{tab:cityscapes_sup}
% \end{table}



% \subsection{Weighting Strategies.} In the main paper, we use the equal weighting for each task. In Table~\ref{tab:weighting}, we show performance with different weighting strategies for the multiple tasks: Uncertainty Weighting~\cite{kendall2018multi} and Dynamic Weight Average~\cite{liu2019end}. These weighting strategies are proposed to find a balance between different tasks, since a model can be biased to a certain task. A desired multi-task learning model should not depend on these weighting schemes, so that the model itself can find a proper balance between tasks. We observe that MILA achieves the similar performance on different weighting strategies and thus is not sensitive to the weighting schemes.


% \begin{table}
% \centering
% \small
% \begin{tabular}[t]{|l|c|c|c|}
% \hline
% Backbone & Weighting & mIOU ($\uparrow$) & Depth Err. ($\downarrow$) \\
% \hline
% \hline
% D101-18 & Equal         &   \textbf{64.3}   &    1.02        \\
% D101-18 & Uncertainty~\cite{kendall2018multi}         &   \textbf{64.3} & \textbf{1.01}  \\
% D101-18 & DWA~\cite{liu2019end}         &  64.2    &  1.02 \\
% % D101-18 & 7x7         &      &            \\
% % D101-18 & Global      &  62.6    & 11.1   \\
% \hline
% \end{tabular}
% % \vskip 0.1in
% \caption{Different weighting strategies for MILA. MILA is not sensitive to the weighting strategies.}
% \label{tab:weighting}
% \end{table}




% \section{Ablation for $Slow$ network-only}
% We apply our full feature propagation method (inter-frame local attention (ILA) + multi-frame feature propagation + task specific) on $Slow$ network-only model. This means that the keyframe interval is 1. Table~\ref{tab:slow-only} shows the results on Cityscapes. In all cases, using our feature propagation method shows significant improvements on the depth estimation task.
% \begin{table}[h]
% \centering
% \small
% \begin{tabular}{|l|c|c|c|c|}
% \hline
% \multirow{2}{*}{Model} & \multicolumn{2}{c|}{Segmentation} & \multicolumn{2}{c|}{Depth}  \\ \cline{2-5}
% & mIOU $\uparrow$ & Acc. $\uparrow$ & Abs.  $\downarrow$ & Rel. $\downarrow$    \\ \hline \hline

% D101-Multi & 63.8 & 94.4 & 1.06 & 31.9 \\
% D101-Multi + Ours & \textbf{64.4} & \textbf{94.6} & \textbf{1.02} & \textbf{25.8} \\
% \hline
% D50-Multi & 63.1 & 94.2 & 1.09 & 33.0 \\
% D50-Multi + Ours & \textbf{63.3} & \textbf{94.5} & \textbf{1.02} & \textbf{25.1} \\
% \hline
% D18-Multi & 60.3 & 93.4 & 1.21 & 34.8 \\
% D18-Multi + Ours & \textbf{61.5} & \textbf{93.8} & \textbf{1.07} & \textbf{25.8} \\
% \hline
% \end{tabular}
% % \vskip 0.1in
% \caption{Evaluation of a Slow-only network with our task-specific inter-frame local attention (ILA) module on Cityscapes.}
% \label{tab:slow-only}
% \end{table}



% \section{Additional Comparison for Feature Propagation}
% In Table~\ref{tab:semantic_segmentation_sup}, we provide more detailed comparisons between our attention based feature propagation and the optical flow based feature warping method by Jain~\etal~\cite{jain2019accel}. We compare the task of video semantic segmentation as in~\cite{jain2019accel}. Our method outperforms~\cite{jain2019accel}, and is more robust to different keyframe interval. Note that we only apply our ILA module for fair comparison with other feature propagation methods (\ie without multi-frame and task-specific attention).

% \begin{table}[h]
% \centering
% \begin{tabular}{|l|c|l|c|}
% \hline
% Backbone & $K$ & Feature Prop. & mIOU (\%) \\
% \hline
% \hline

% % \hline
% % \hline
% % D50 & 1 & \multicolumn{1}{c|}{-} & 70.1 \\
% % \hline
% D101-50 & 5 & Optical flow & 74.2 \\
% D101-50 & 5 & ILA (Ours) & \textbf{75.1}\\
% \hline
% D101-50 & 10 & Optical flow & 72.9 \\
% D101-50 & 10 & ILA (Ours) & \textbf{74.8} \\
% % \hline
% \hline
% % DANet101 & 1 & \multicolumn{1}{c|}{-} & 81.5 \\
% % DANet101 & 1 & Ours (LA) & \textbf{81.6}\\
% % \hline
% \end{tabular}
% % \vskip 0.1in

% \caption{Supplements to Table~5 in the main paper. Comparison with optical-flow based feature propagation~\cite{jain2019accel} for the semantic segmentation task on Cityscapes. A keyframe interval is denoted by $K$. We show detailed comparison using different backbones and keyframe intervals.}
% \label{tab:semantic_segmentation_sup}
% \end{table}


% \section{Additional Qualitative Results}
% In the main paper, we only put the qualitative results on Cityscapes due to the limited space. We also provide the qualitative results on NYU v2 in Figure~\ref{fig:qualitative_nyu}. Compared to MultNet++~\cite{chennupati2019multinet++}, our method is robust to non-keyframes and obtains similar performances as the computationally heavy method~\cite{liu2019end}. In addition, we also provide the supplemental video of predictions of the $Slow$ and $Fast$ networks, where the $Fast$ network produces qualitatively similar performances as the $Slow$ network.

% \begin{figure*}[t]
% 		\centering
% 		\includegraphics[width=1.0\linewidth]{fig_qualitative_nyu.pdf} 
% 		\vskip -0.1in
% 		\caption{Qualitative results for multi-task learning on videos on the NYUd v2 dataset. We show comparison between (a) MultiNet++, (b) MTAN and (c) ours. MultiNet++ performs worse on the non-keyframe. }
% 		\label{fig:qualitative_nyu}
% \end{figure*}


% \section{Discriminator Details}
% The discriminator $D$ takes feature maps from the last residual block of slow and fast network. The discriminator consists of three 3x3 convolutional layers with relu activtaion, a global average pooling layer, and sigmoid activation, which outputs a single value. It should be noted that the discriminator is only used during training, therefore it does not increase GFLOPs in inference time. [R4] We update the encoder and discriminator jointly by using a gradient-reversal layer~\cite{ganin2016domain} for Eq.~3.

% {\small
% \bibliographystyle{ieee_fullname}
% \bibliography{egbib}
% }

% \end{document}
